# Supplementary material for: The Bulk and The Tail of Minimal Absent Words in Genome Sequences
Source: arXiv:1509.05188 ancillary file (2015-09-17)
Supplement: Supplementary file 1 [file Supplemental_Information.pdf]

# The Bulk and The Tail of Minimal Absent Words in Genome Sequences

# Supplementary Information

Erik Aurell[1,2], Nicolas Innocenti[1] and Hai-Jun Zhou[3]

[1]Department of Computational Biology, KTH Royal Institute of Technology, AlbaNova University Center, SE-10691 Stockholm, Sweden

[2]Department of Information and Computer Science, Aalto University, FI-02150 Espoo, Finland

[3]State Key Laboratory of Theoretical Physics, Institute of Theoretical Physics, Chinese Academy of Sciences, Beijing 100190, China

## Appendix A. Minimal absent words formed by a single letter

The probabilistic theory of the main text assumes that each MAW is formed by at least two letters. Here we consider the special case of a word $\mathbf{w} = c_1 c_2 \dots c_L$ of length $L$ composed of a single letter, *i.e.* $c_1 = c_2 = \dots = c_L = c$. The two $(L-1)$ long subwords of such a word are identical, $\mathbf{w}^{(p)} = \mathbf{w}^{(s)}$. For such a special word $\mathbf{w}$ to be a MAW it must not be a word of $\mathcal{S}$ but its prefix $\mathbf{w}^{(p)}$ (equivalently, the suffix $\mathbf{w}^{(s)}$) must be a word of $\mathcal{S}$. Therefore we can write down the probability $q_{\mathbf{w}}$ of $\mathbf{w}$ being a MAW as

$$q_{\mathbf{w}} = \left(1 - \omega_c^L\right)^{N-L+1} - \left(1 - \omega_c^{L-1}\right)^{N-L+2} . \tag{1}$$

We have confirmed the good performance of Eq. 1 by computer simulations (see comparative results in Fig. SA). The expected length of this special MAW is

$$\langle L \rangle = \sum_{L \geq 1} L q_{\mathbf{w}} \simeq \sum_{k=0}^{N} \left[1 - \left(1 - \omega_c^k\right)^{N-k+1}\right] . \tag{2}$$

We find that this mean length $\langle L \rangle$ is very close to the most probable length (corresponding to the maximum of $q_{\mathbf{w}}$) and it increases with the total sequence length $N$ as

$$\langle L \rangle \approx -\frac{\ln N}{\ln \omega_c} . \tag{3}$$

Notice that any genetic sequence $\mathcal{S}$ has only four such special MAWs, namely $A \dots A$, $C \dots C$, $G \dots G$ and $T \dots T$, therefore they can be neglected as long as the total number of MAWs is concerned. These four special MAWs are not considered in the main text.

## Appendix B. Probabilistic estimate of shortest absent words

In this Appendix we derive a general probabilistic estimate for the shortest absent words in a random text, adapting a classic analysis of intergalactic voids [46], see also Appendix A of [47].

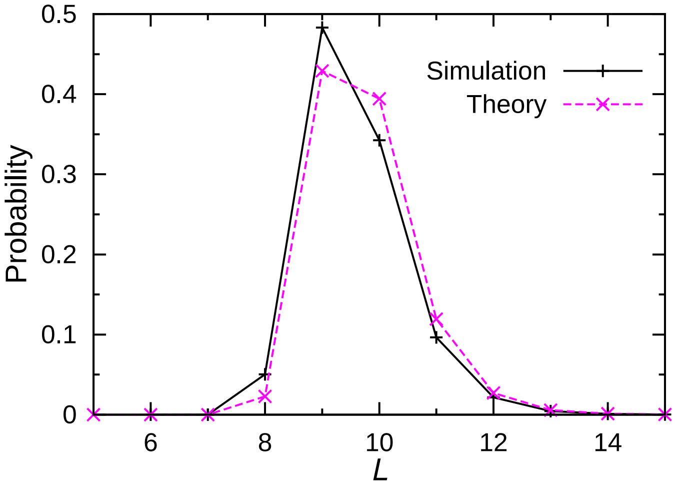


Figure SA: Probability of a length-$L$ special word $\mathbf{w} = GG \dots G$ being a minimal absent word of a random genetic sequence $\mathcal{S}$. The $+$ symbols are results from computer simulations, while the $\times$ symbols are the predictions of the mean-field theory (Eq. 1 above). The length of the random sequence $\mathcal{S}$ is $N = 10^6$ and the fraction of letter $G$ in the sequence is $\omega_G = 0.21$.

As the shortest absent words are necessarily minimal this analysis also applies to shortest minimal absent words.

We start by defining $F_1(\mathbf{w_1}; T)$ to be the probability that word $\mathbf{w_1}$ is absent from a text $T$. Similarily, for $n > 1$ we define $F_n(\mathbf{w_1}, \mathbf{w_2}, \dots, \mathbf{w_n}; T)$ to be the probability that the $n$ words $\mathbf{w_1}, \dots, \mathbf{w_n}$ are all absent from $T$. Note that this definition makes no reference to other words which could be either absent or present. If any two words in the argument happen to be the same we define such an $F_n$ to be zero; no word can be absent twice. The expected number of words in a collection of words $C$ that are absent in $T$ is $f_1(C; T) = \sum_{\mathbf{w} \in C} F_1(\mathbf{w}; T)$. Similarly we introduce the quantities

$$f_n(C, T) = \sum_{\mathbf{w_1} \in C, \dots, \mathbf{w_n} \in C} F_n(\mathbf{w_1}, \mathbf{w_2}, \dots, \mathbf{w_n}; T). \tag{4}$$

We also define $f_0(C, T) = 1$. We then proceed by defining $P_1(\mathbf{w_1}; T)$ to be the probability that word $\mathbf{w_1}$ is absent and all other words present. For $n > 1$ we define $P_n(\mathbf{w_1}, \mathbf{w_2}, \dots, \mathbf{w_n}; T)$ to be the probability that the $n$ words $\mathbf{w_1}, \dots, \mathbf{w_n}$ are all absent, and all other words present. If any two words in the argument are the same we define such a $P_n$ to be zero. The probability that there are precisely $n$ (different) words absent is then

$$p_n(C, T) = \frac{1}{n!} \sum_{\mathbf{w_1} \in C, \dots, \mathbf{w_n} \in C} P_n(\mathbf{w_1}, \mathbf{w_2}, \dots, \mathbf{w_n}; T), \tag{5}$$

where the factorial takes care of permutations. From here on we will only consider collections $C$ consisting of all words of length $l$, and we will for brevity supress the dependence on $T$. What we are interested in is the probability that there are no words absent in a collection of words of length $l$ *i.e.*

$$p_0(l) = 1 - p_1(l) - p_2(l) - \cdots \ . \tag{6}$$

We expect $p_0(l)$ to decrease smoothly from $p_0(1) \approx 1$ to $p_0(L) = 0$ if $4^L$ is larger than the length of the text, and we can define a predictor $l^*$ to be the integer such that $p_0(l^*)$ is closest to $\frac{1}{2}$.

The probability that word $\mathbf{w_1}$ is absent must be the same as the probability that it is the only absent word plus the probability that it is one out of two only absent words, and so on. Expressed

in the quantities defined above this means

$$F_1(\mathbf{w_1}) = P_1(\mathbf{w_1}) + \sum_{\mathbf{w_2}} P_2(\mathbf{w_1},\mathbf{w_2}) + \frac{1}{2!}\sum_{\mathbf{w_2},\mathbf{w_3}} P_3(\mathbf{w_1},\mathbf{w_2},\mathbf{w_3}) + \cdots \ , \tag{7}$$

and similarly

$$F_n(\mathbf{w_1},\ldots,\mathbf{w_n}) = \sum_{l=0}^{\infty}\frac{1}{l!}\sum_{\mathbf{w'_1},\ldots,\mathbf{w'_l}} P_{n+l}(\mathbf{w_1},\ldots,\mathbf{w_n},\mathbf{w'_1},\ldots,\mathbf{w'_l}). \tag{8}$$

Summing (8) over all the words $\mathbf{w_1},\ldots,\mathbf{w_n}$ we obtain

$$f_n = n!p_n + \frac{(n+1)!}{1!}p_{n+1} + \frac{(n+2)!}{2!}p_{n+2} + \cdots \ . \tag{9}$$

Multiplying (9) by $(-)^n/n!$ and summing over $n$ we obtain

$$p_0 = \sum_{n=0}^{\infty}\frac{(-)^n}{n!}f_n. \tag{10}$$

If the probabilities of words to be absent would be independent we would have $F_n(\mathbf{w_1},\ldots,\mathbf{w_n}) = \prod_{l=1}^{n} F_1(\mathbf{w_l})$ and $p_0 = \exp(-f_1)$. To proceed further we have to take correlations between different words to be absent into account, and following [46] we do so by recursively introducing a cluster expansion

$$\begin{aligned}
F_1(\mathbf{w_1}) &= C_1(\mathbf{w_1}) \\
F_2(\mathbf{w_1},\mathbf{w_2}) &= C_1(\mathbf{w_1})C_1(\mathbf{w_2}) + C_2(\mathbf{w_1},\mathbf{w_2}) \\
&\vdots \\
F_n(\mathbf{w_1},\ldots,\mathbf{w_n}) &= \sum_{\text{partitions}} \cdots C_l(\mathbf{w_{r_1}},\ldots,\mathbf{w_{r_l}})\cdots \ ,
\end{aligned}$$

and associated cumulants

$$c_n = \sum_{\mathbf{w_1},\ldots,\mathbf{w_n}} C_n(\mathbf{w_1},\mathbf{w_2},\ldots,\mathbf{w_n}). \tag{11}$$

Comparing (9) and (11) we have the final formula

$$p_0 = \exp\left(\sum_{n=1}^{\infty}\frac{(-)^n}{n!}c_n\right). \tag{12}$$

We note that the first term in this sum gives the same estimate as if the probabilities of words to be absent were independent, since

$$c_1 = f_1 = \sum_{\mathbf{w}} F_1(\mathbf{w}). \tag{13}$$

We further note that for two copies of the same word we always have

$$C_2(\mathbf{w},\mathbf{w}) = -(F_1(\omega))^2, \tag{14}$$

which gives a part of second term in the exponent in (12) as

$$c_2^{\text{diag}} = -\sum_{\mathbf{w}}(F_1(\mathbf{w}))^2. \tag{15}$$

Given (12) it is natural to define a full estimate of $l^*$ as the integer $l$ such that $c_1(l) - \frac{1}{2}c_2(l) + \ldots$ is as close as possible to $\log 2$. In practice we however expect $c_2^{\text{diag}}$ and all higher corrections to be small, so that a prediction for $l^*$ can be based on $c_1$. In the main text and below we have used the estimate that $f_1(l) = c_1(l)$ is as close as possible to one, which is practice gives the same result as $c_1(l) = \log 2$.

## Appendix C. Comparisons of shortest absent words on a test set

From the previous section a general predictor for the shortest absent word is

$$l^* = \arg\min_l |f_1(l) - 1|, \tag{16}$$

where $f_1(l)$ is given by (13). From this it is clear that the basic elements are estimates of $F_1(\mathbf{w})$, the probability that a given word is absent. In the main text we have used the estimate ("Varying", implicit in Eqs 1 and 4)

$$F_1^{\rm var}(\mathbf{w}) = [1 - \omega(\mathbf{w})]^{N-L+1}, \qquad \omega(\mathbf{w}) = \prod_{i=1}^{L} \omega_{c_i}, \tag{17}$$

which (as stated there) ignores interactions between words. We have also used a simpler estimate ("uniform", implicit in Eq 3) which additionally ignores the dependence on nucleotide composition *i.e.* simplifies (17) by taking $\omega(\mathbf{w}) = 4^{-L}$ for all words of length $L$. The uniform estimate has the advantage that the minimization can be carried out analytically, and in practice we then use the real-valued approximation $l^* \approx \frac{\ln N - \ln\ln N}{\ln 4}$ (Eq. 6). In the only other analysis of shortest absent words that we are aware of [17], the quantity $F_1(\mathbf{w})$ is estimated by a Poisson argument to be

$$F_1^{\rm Wu}(\mathbf{w}) = e^{-N\omega(\mathbf{w})}. \tag{18}$$

This same estimate was earlier stated in [14], but not used therein. These two estimates in (17) and (18) are related by

$$F_1^{\rm var}(\mathbf{w}) = F_1^{\rm Wu}(\mathbf{w}) e^{-N\frac{1}{2}(\omega(\mathbf{w}))^2 + \dots}, \tag{19}$$

which means that the two estimates of $f_1$ are related by

$$f_1^{\rm var} = f_1^{\rm Wu} - \frac{1}{2N} \sum_{\mathbf{w}} e^{-N\omega(\mathbf{w})} (N\omega(\mathbf{w}))^2 + \text{h.o.t.}\ . \tag{20}$$

For the relevant lengths $f_1$ should be of order unity, and for unbiased genomes this means $N\omega(\mathbf{w}) \approx L \log 4$. The correction term in (20) is then approximately $L^2/N$ and would vanish for sufficiently long texts. For very biased genomes the two estimates of $F_1$ in (17) and (18) may on the other hand give different predictions for $l^*$.

In Table 1 we give predicted length of the shortest absent words for the same set of organisms considered by Wu et al. [17], and earlier by Herold et al. [14]. Note that in the main text we consider (Fig. 4) a far larger set of genomes and find that the true length of the shortest absent words fluctuate around these estimates by $\pm 2$. Indeed, given that the occurrences of nearby nucleotides are not independent but can be modeled by $k$-order Markov chains, better estimates of $F_1(\mathbf{w})$ could be obtained, and we do not expect estimates built only on single nucleotide frequencies to be exact. We find that our simplest estimate (column "Uniform", Eq. 6 in main text) is already reasonable, differing by one to three nucleotides in length for all the genomes in this list. Our more precise estimate (column "Varying", Eq 4 in main text) is overall better, and agrees with the truth for four out of ten entries.

Using the estimate in [17] on the same data we find (column "ESW estimate") complete agreement with our "Varying" estimate, as one would expect from the above discussion since none of these genomes is very biased. We note that the numbers published in [17] (column "Wu et al") are different from what we get using the same method, agreeing with the truth in six cases out of ten (it additionally agrees with the truth for *C. elegans*, *T. kodakarensis* and *S. aureus*, but instead does not agree for *M. genitalium*). As the paper [17] was published in 2010 the discrepancy can be due to the use of different genome assemblies, but unfortunately we cannot conclude this with certainty based on the information given in [17]. Another possibility, based on the name given to

one of the input variables in the publicly available implementation of the algorithm in [17], is that the numbers in [17] (column "Wu et al") might have been computed using the genome length, while the data (column "Truth") has been computed from both strands of the genome, a text of twice that length [1]. In any case, as argued above we cannot expect predictions based on single nucleotide frequencies to be exact, and the predictions in the columns "Varying", "ESW estimate" and "Wu et al" in Table 1 are clearly all very good.

# References


[14] Herold, J, Kurtz, S, & Giegerich, R. (2008) Efficient computation of absent words in genomic sequences. *BMC Bioinformatics* **9**, 167.

[17] Wu, Z.-D, Jiang, T, & Su, W.-J. (2010) Efficient computation of shortest absent words in a genomic sequence. *Information Processing Letters* **110**, 596 – 601.

[46] Balian, R & Schaeffer, R. (1989) Scale-invariant matter distribution in the universe. *Astron. Astrophys.* **220**, 1–29.

[47] Gurbatov, S. N, Simdyankin, S. I, Aurell, E, Frisch, U, & Tóth, G. (1997) On the decay of burgers turbulence. *Journal of Fluid Mechanics* **344**, 339–374.


[1] We have observed that using the genome length as input to the estimate in [17], instead of twice the genome length as in the table where we considered double-stranded genomes, improves the agreement to column "Wu et al" in Table 1, although not to perfect concordance.

| Organism | Genome Size | GC content (%) | Uniform | Varying | ESW estimate | Wu et al. | Truth | Nb. shortest AW |
|---|---|---|---|---|---|---|---|---|
| Human | 2.9 G | 41.0 | 13.9 | 12 | 12 | 12 | 11 | 104 |
| Mouse | 2.6 G | 41.7 | 13.8 | 12 | 12 | 12 | 11 | 184 |
| *D. melanogaster* | 120 Mbp | 42.4 | 11.8 | 11 | 11 | 11 | 11 | 182 |
| *C. elegans* | 100 Mbp | 35.4 | 11.7 | 9 | 9 | 10 | 10 | 2 |
| *N. crassa* | 40.0 Mbp | 48.9 | 11.0 | 11 | 11 | 11 | 11 | 1980 |
| *S. cerevisiae* | 12.1 Mbp | 38.3 | 10.2 | 9 | 9 | 9 | 9 | 4 |
| *S. aureus* | 2.82 Mbp | 32.8 | 9.23 | 7 | 7 | 8 | 8 | 225 |
| *T. kodakarensis* | 2.09 Mbp | 52.0 | 9.03 | 9 | 9 | 8 | 8 | 1 |
| *M. jannaschii* | 1.74 Mbp | 31.3 | 8.91 | 7 | 7 | 7 | 6 | 2 |
| *M. genitalium* | 580 kbp | 31.7 | 8.17 | 6 | 6 | 7 | 6 | 3 |

Table 1: Estimation of the length of the shortest absent words for the same set of species as in Table 2 in Herold et al. [14] and Table 1 in Wu et al. [17]. The *Uniform* estimate uses Eq 6 in main text while the *Varying* estimate uses Eq 4 in main text *i.e.* the criterion (16) combined with the estimate (17). Both strands of the genome are considered in each case. The ESW estimator is obtained from the publicly available implementation of "algorithm 2" from Wu et al. [17], while he column *Wu et al.* shows the results from Table 1 in that paper. Given the publication date of [17] these latter numbers must, for some of these organisms, have been computed from different versions of the genomes.

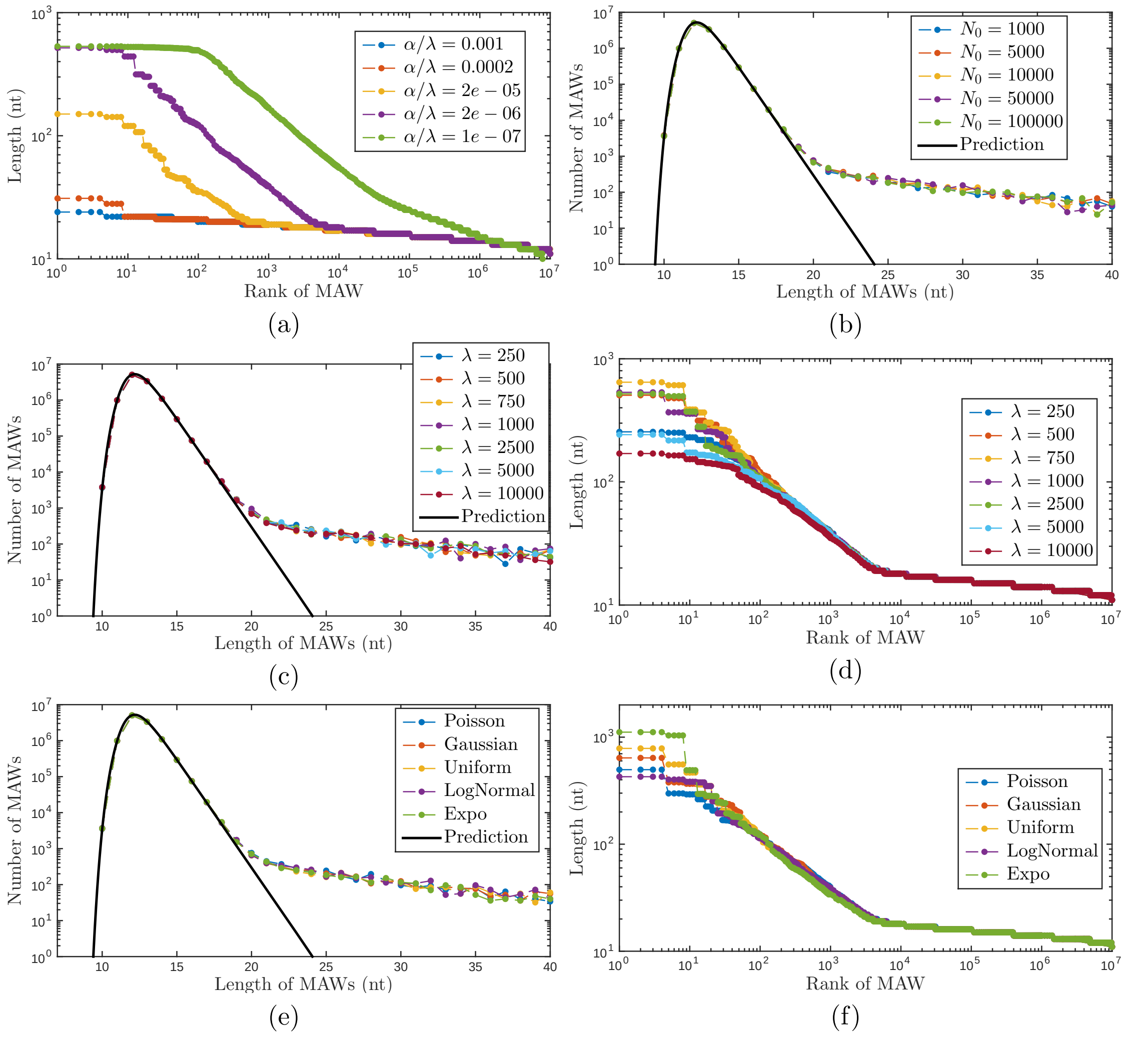


Figure S1: Distributions of MAWs for random genomes generated using the copy-paste-mutate protocol detailed in the main text. Unless other values are specified, the parameters used in all the figures are $\lambda = 1000$, $N_0 = 5000$, $\alpha/\lambda = 2\ 10^{-6}$, uniform probability of letters for the mutations and a final genome size of $3\ 10^6$ bp. (a) shows the same data as in Fig 3 in the form of a rank plot showing the length of a MAW as a function of its rank after ordering all the MAWs from the largest to the smallest. (b) shows that the distributions are not sensitive to the size $N_0$ of the initial fragment (provided that it is much smaller than the final genome length). (c) and (d) show the distributions obtained for genomes generated using different values for $\lambda$ while keeping the a constant ratio $\alpha/\lambda = 2\ 10^{-6}$. The value of $\lambda$ affects only the MAWs far from the bulk. (e) and (f) show the results obtained with different random distributions for the size of the region to be copy-pasted. The numbers are rounded to the nearest integer for continuous probability distributions. The parameters are chosen so that the mean is $\lambda = 1000$ in every case. The distribution used are Poisson, Gaussian with variance $\lambda$, uniform in the range $[0, 2\lambda]$, log normal with variance $\lambda$ and exponential.

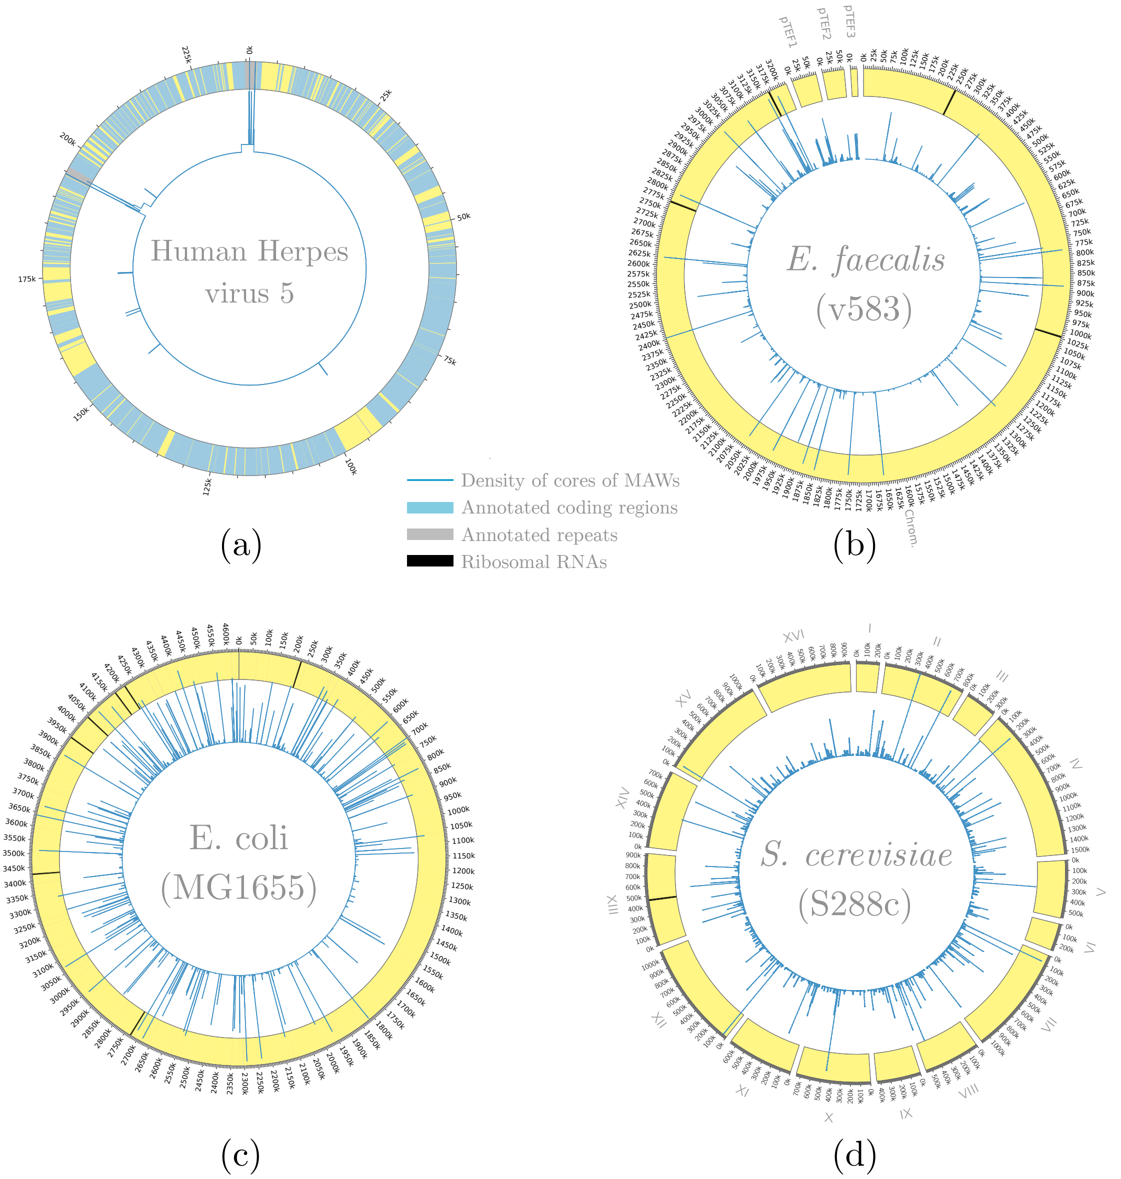


Figure S2: Distribution of cores of MAWs from the tail in (a) the Human Herpes virus 5 (strain Merlin), (b) *E. faecalis* (strain v583), (c) *E. coli* (strain MG1655) and (f) *S. cerevisiae* (strain S288C). The inner plots represent the number of cores of MAWs covering the corresponding position.
